# Supplementary material for: Effect of negative triangularity on SOL plasma turbulence in double-null L-mode plasmas
Source: arXiv:2412.20780 source file (2024-12-30)
Supplement: Supplementary file 1 [file 8_Appendix.tex]

\section{Appendix}\label{Appendix:1}
\par\noindent\rule{\textwidth}{0.4pt}

\begin{itemize}
    \item Reduced connection length in NT plasmas. The parallel connection length $L_\parallel$ is strongly reduced in negative triangularity. From the context of the two-region model, this can be related to a change in filamentary regime. In fact, for the very short parallel connection lengths measured, filaments are expected to be in the $C_s$ regime, in which parallel currents can efficiently short-circuit the poloidal potential within the filaments. \textcolor{red}{(Usually, NT plasmas are known for a reduced connection lengths, however, in the present simulations, the parallel connection length between PT and NT do not see a big differences, as they are simply flipped.)}
    \item \textcolor{red}{The effect of finite ion temperature}, which is important, is addressed in Ref.\,\cite{Jovanovic2008} + \textcolor{red}{Parallel electron dynamics}. In this work, it shows that the effects of the finite ion temperature and the parallel resistivity introduces the symmetry breaking of blobs, as compared with their 2D, cold ion counter parts.
    \item Other works in Blobs, but using the cold ion approximation \cite{Sarazin1998, Bisai2004, Yu2006}
    \item The filamentary structure of the SOL also has implications for radio-frequency plasma (RF) heating schemes. The wavelength of the incoming RF waves is similar enough to the size of and spacing between the filaments that they are strongly diffracted as they pass through the SOL, reducing the precision of the heating \cite{Myra2010, Brookman2021}.
    \item Pressure gradients within these filaments create diamagnetic currents, which are closed partially by polarization currents. The latter create electric fields across the filaments in the drift-plane, which drive filaments radially outwards through $\bm{E} \times \bm{B}$ drifts. \textcolor{red}{Okay, but this physical mechanisms is less relevant with my cases}
    \item D'Ippolito describes filament formation as a process of long \textit{streamers} being formed from instabilities, which are cut-off by velocity shear in the fluid. In this model, a shearless fluid produces long streamers, moderate shear would create filaments like those in L-mode, and strong shear would break up filaments quickly and suppress transport, as in H-mode. \textcolor{red}{(This is a more linked with my cases, need to read all the related literature and cite them, providing a clear physical mechanism why NT has smaller and slower blobs.)}
    \item Plasma density blobs form in the edge or in the edge-to-SOL transition region where the poloidal velocity shear is maximum. Typically, the blob formation events are related to the breaking of the radially elongated streamers under the action of the differential velocity shear.
    \item In other experiments with TORPEX, it has shown that the radially elongated structure responsible for the blob formation are associated with the destabilization of tinterchange waves in the presence of velocity shear \cite{Furno2008} along the lines of the mechanism proposed in Ref. \cite{Bisai2005}
    \item The origin of zonal flow leads to a strong velocity shear that moves different parts of the density streamer structure at different velocities in the poloidal direction giving rise to a net displacement among different parts of the structure. If this net displacement is grater than the poloidal width $\delta_y$ of the streamer then the streamer will be broken and the broken part will form a blob
    \item The blob formation mechanisms proposed by Bisai is premised on the existence of a density streamer structure and its subsequent breakup by the velocity shears.
    \item Blobs are the result of the nonlinear saturation of interchange-like instabilities in the edge, with the density flcutuation sheared apaart by the $E \times B$ velocity and detached from the main plasma, as observed in JET \cite{Xu2009} and TORPEX \cite{Furno2008}
    \item The list of TCV blob works, the characterization of blobs based on two-region model from TCV experimental observations in \cite{Offeddu2022}
    \item The structure can break if the temporal shearing rate is faster than the temporal growth rate $\gamma$ of the streamer due to the background interchange instability.
    \item For diverted plasmas, recent work \cite{Carralero2015} suggests that the collisionality in the divertor $\Lambda_{\textrm{div}}$ is more important than $\Lambda_{\textrm{mid}}$.
    \item on the effects of magnetic geometry, such as the presence of X-point and its impact on tilting (squeezing) the blobs when passing near by due to the magnetic expansion \cite{Farina1993}. Although the effects of various magnetic configurations have been investigated experimentally, particularly in TCV tokamaks \cite{Han2021} indicating reduced interaction between plasma and the first wall, 
    \item It should also be noted that the effects of plasma shaping on boundary plasma turbulence mainly arise from the geometrical operators in GBS in Eqs.~(\ref{GBS_operator1}--\ref{GBS_operator4}). In particular, the curvature operator in the LFS region is strongly affected by triangularity, thereby altering the level of RBMs instabilities between NT and PT plasmas, as outlined with the SN configurations in Ref.~\cite{Lim2023}.
    \item Cross-field transport of particles in the SOL region is primarily dominated by the radial outward motion of coherent plasma structures, called blobs. The presence of blobs is ubiquitous, occurring in various tokamaks \cite{Boedo2001, Terry2003, Goncalves2005, Zweben2007, Garcia2007, Tanaka2009, Fedorczak2009, Birkenmeier2014, Vianello2020}, basic plasma experiments \cite{Furno2008, Muller2009, Theiler2009, Manz2011}, linear devices \cite{Carter2006, Pace2008}, reversed field pinches \cite{Antoni2001, Cavazzana2007, Vianello2016}, and stellarators \cite{Dewhurst2008, Happel2009}. Curvature and $\nabla B$ drifts inside the blob drive vertical charge separation within the blobs, inducing $E \times B$ drift that advects the blobs radially outward \cite{Krasheninnikov2001, Ippolito2002}.  This phenomenon has been evidenced by numerical simulations with seeded blobs \cite{Militello2013, Halpern2014, Riva2016}, showing that particle and heat flux in the far SOL region is dominated by the radial propagation of blobs. Therefore, understanding blob dynamics is particularly important to mitigate these deleterious interactions with the first walls \cite{Ippolito2002}.
    \item \textcolor{red}{(In RB regimes, blobs are not connected to the divertor regions, like in NT cases. However, in PT 2D snapshot, we see some blobs under the X-point, which means that they are connected at some point, probably in RX regime. Verify it).}
    \item The application of two-region model have been tested and represent un upper boundary of for the radial propagation velocity of filaments \cite{Theiler2009, Tsui2018}
    \item In the upstream region, the unfavourable curvature of the magnetic field leads to the formation of an electric dipole that provides mos of the drive for the blob radial motion. In the divertor region, the magnetic flux expansion causes the blob to elongate in one direction and squeeze in the other.
    \item In L-mode plasma, which is characterized relatively high plasma resistivity, the strong resistivity of plasma opposes the flow of electric current from upstream to the target plates. Therefore, the current is mainly by ion polarization current before they enter the divertor regions. The effect of plasma resistivity on filamentary dynamics is outlined in Ref. \cite{Easy2014}, showing that strong resistivity affects the extended to which these parallel currents can flow. The influence of parallel resistivity on the dynamics of filaments has previously been considered theoretically by Ref. \cite{Myra2006}. Increased collisionality will lead to an increase in filament velocities and hence turbulence transport, whilst increased magnetic field line fanning and shear has the opposite effect.
    \item In addition to the power exhaust challenge in fusion devices, cross-field transport in the scrape-off layer (SOL) region presents a critical issue that must be addressed. This transport is primarily driven by the radial outward motion of coherent plasma structures known as blobs. Understanding blob dynamics is crucial because strong interactions between blobs and the first wall can lead to sputtering and erosion of wall components, posing significant concerns for the operation of fusion devices \cite{Ippolito2002}. Over the past decades, extensive studies have been carried out on blob dynamics from both numerical and theoretical perspectives, as detailed in comprehensive review in Ref.~\cite{Ippolito2011}. These studies encompass a range of approaches, from simplified 2D models and cold-ion approximations to considerations of finite Larmor radius (FLR) effects and blob seeding in three-dimensional analyses. However, since blob interactions with a three-dimensional background turbulence plasma are crucial for accurately determining blob dynamics \cite{Angus2012, Walkden2013, Easy2014}, a thorough analysis inherently requires a self-consistent and three-dimensional treatment of plasma turbulence. Three-dimensional blob dynamics have been addressed by various codes, such as BOUT++ \cite{Russell2004}, GBS \cite{Nespoli2017, Paruta2019}, and GRILLIX \cite{Ross2019, Zholobenko2023}, which show consistent behavior with theoretical predictions. Despite these extensive studies, a clear explanation of the effects of triangularity on blob dynamics remains elusive and has not yet been provided by any boundary plasma turbulence code.
\end{itemize}
